# Supplementary material for: Learning Keypoints for Robotic Cloth Manipulation using Synthetic Data
Source: arXiv:2401.01734 source file (2024-05-21)
Supplement: Supplementary file 1 [file appendices.tex]

\appendices
\section{Dataset Details}
Appendix one text goes here.
\section{Keypoint Detector Details}
Appendix two text goes here.
\section{ProcGent Details}
Randomization ranges etc. 

\section{Engineering Findings}

A few things I would like to write down for myself. Probably don't belong in the paper.

Recipe for Sim2real? it is often manual trial and error (e.g. https://developer.nvidia.com/blog/closing-the-sim2real-gap-with-nvidia-isaac-sim-and-nvidia-isaac-replicator/), but still there are some guidelines to follow maybe and some metrics to watch?

Architecture of a synthetic data generation pipeline:
how to manage the randomization parameters and the diverse 'options' for different aspects of the pipeline.
